# Supplementary material for: ExoTST: Exogenous-Aware Temporal Sequence Transformer for Time Series Prediction
Source: arXiv:2410.12184 source file (2024-10-16)
Supplement: Supplementary file 1 [file appendix.tex]

\section{Appendix}
\subsection{Full Results}\label{appendix:flux_tower_results}

\begin{table}[H]
\caption{Full results of the long-term forecasting task with exogenous drivers. The lowest MSE for each horizon and dataset is \textbf{emphasized} in bold.}
\vspace{2pt}
\setlength{\tabcolsep}{2.5pt}

\begin{sc}
\resizebox{\linewidth}{!}{
\begin{tabular}{c|c|cc|cc|cc|cc|cc|cc|cc|cc}
\toprule[1.2pt]  
\multicolumn{2}{c}{\multirow{2}{*}{\scalebox{1.35}{Models}}}   & \multicolumn{2}{c}{\scalebox{1.35}{FutureTST}} & \multicolumn{2}{c}{\scalebox{1.35}{iTrans.}} & \multicolumn{2}{c}{\scalebox{1.35}{(U)PatchTST}} & \multicolumn{2}{c}{\scalebox{1.35}{(M)PatchTST}} & \multicolumn{2}{c}{\scalebox{1.35}{LSTM}} & \multicolumn{2}{c}{\scalebox{1.35}{DLinear} }& \multicolumn{2}{c}{\scalebox{1.35}{TiDE}} & \multicolumn{2}{c}{\scalebox{1.35}{S-Mamba}} \\ 
\multicolumn{2}{c}{} & \multicolumn{2}{c}{\scalebox{1.35}{(Ours)}} & \multicolumn{2}{c}{\scalebox{1.35}{\citeyearpar{liu2023itransformer}}} & \multicolumn{2}{c}{\scalebox{1.35}{\citeyearpar{nie2022time}}} & \multicolumn{2}{c}{\scalebox{1.35}{\citeyearpar{nie2022time}}} & \multicolumn{2}{c}{\scalebox{1.35}{\citeyearpar{yin2022rr}}} & \multicolumn{2}{c}{\scalebox{1.35}{\citeyearpar{zeng2023transformers}}} & \multicolumn{2}{c}{\scalebox{1.35}{\citeyearpar{das2023long}}} & \multicolumn{2}{c}{\scalebox{1.35}{\citeyearpar{wang2024mamba}}}\\ 
\cmidrule(lr){3-4}\cmidrule(lr){5-6}\cmidrule(lr){7-8}\cmidrule(lr){9-10}\cmidrule(lr){11-12}\cmidrule(lr){13-14}\cmidrule(lr){15-16}\cmidrule(lr){17-18}
\multicolumn{2}{c}{\scalebox{1.35}{Metric}}   & \scalebox{1.35}{MSE} & \scalebox{1.35}{MAE} & \scalebox{1.35}{MSE}    & \scalebox{1.35}{MAE}   & \scalebox{1.35}{MSE}    & \scalebox{1.35}{MAE}    & \scalebox{1.35}{MSE}    & \scalebox{1.35}{MAE} & \scalebox{1.35}{MSE}    & \scalebox{1.35}{MAE} & \scalebox{1.35}{MSE}    & \scalebox{1.35}{MAE}   & \scalebox{1.35}{MSE}    & \scalebox{1.35}{MAE}  & \scalebox{1.35}{MSE}    & \scalebox{1.35}{MAE}      \\ 
\toprule[1.2pt] 
\multirow{5}{*}{\scalebox{1.35}{\rotatebox{90}{DE-HAI}}}
 & \scalebox{1.35}{30} & \scalebox{1.35}{\textbf{0.079}} & \scalebox{1.35}{0.194} & \scalebox{1.35}{0.082} & \scalebox{1.35}{0.197} & \scalebox{1.35}{0.089} & \scalebox{1.35}{0.214} & \scalebox{1.35}{0.089} & \scalebox{1.35}{0.210} & \scalebox{1.35}{0.140} & \scalebox{1.35}{0.284} & \scalebox{1.35}{0.093} & \scalebox{1.35}{0.220} & \scalebox{1.35}{0.098} & \scalebox{1.35}{0.228} & \scalebox{1.35}{0.238} & \scalebox{1.35}{0.378}\\
 & \scalebox{1.35}{60} & \scalebox{1.35}{\textbf{0.084}} & \scalebox{1.35}{0.201} & \scalebox{1.35}{0.095} & \scalebox{1.35}{0.222} & \scalebox{1.35}{0.097} & \scalebox{1.35}{0.221} & \scalebox{1.35}{0.098} & \scalebox{1.35}{0.222} & \scalebox{1.35}{0.148} & \scalebox{1.35}{0.292} & \scalebox{1.35}{0.104} & \scalebox{1.35}{0.239} & \scalebox{1.35}{0.106} & \scalebox{1.35}{0.238} & \scalebox{1.35}{0.115} & \scalebox{1.35}{0.240}\\
 & \scalebox{1.35}{90} & \scalebox{1.35}{\textbf{0.095}} & \scalebox{1.35}{0.221} & \scalebox{1.35}{0.109} & \scalebox{1.35}{0.246} & \scalebox{1.35}{0.106} & \scalebox{1.35}{0.236} & \scalebox{1.35}{0.105} & \scalebox{1.35}{0.236} & \scalebox{1.35}{0.158} & \scalebox{1.35}{0.303} & \scalebox{1.35}{0.109} & \scalebox{1.35}{0.249} & \scalebox{1.35}{0.113} & \scalebox{1.35}{0.248} & \scalebox{1.35}{0.150} & \scalebox{1.35}{0.299}\\
 & \scalebox{1.35}{120} & \scalebox{1.35}{\textbf{0.115}} & \scalebox{1.35}{0.251} & \scalebox{1.35}{0.126} & \scalebox{1.35}{0.274} & \scalebox{1.35}{0.127} & \scalebox{1.35}{0.267} & \scalebox{1.35}{0.122} & \scalebox{1.35}{0.260} & \scalebox{1.35}{0.164} & \scalebox{1.35}{0.311} & \scalebox{1.35}{0.126} & \scalebox{1.35}{0.264} & \scalebox{1.35}{0.118} & \scalebox{1.35}{0.255} & \scalebox{1.35}{0.122} & \scalebox{1.35}{0.258}\\
\cmidrule(lr){2-18}
 & \scalebox{1.35}{AVG} & \scalebox{1.35}{\textbf{0.093}} & \scalebox{1.35}{0.217} & \scalebox{1.35}{0.103} & \scalebox{1.35}{0.235} & \scalebox{1.35}{0.105} & \scalebox{1.35}{0.235} & \scalebox{1.35}{0.103} & \scalebox{1.35}{0.232} & \scalebox{1.35}{0.153} & \scalebox{1.35}{0.297} & \scalebox{1.35}{0.108} & \scalebox{1.35}{0.243} & \scalebox{1.35}{0.109} & \scalebox{1.35}{0.242} & \scalebox{1.35}{0.156} & \scalebox{1.35}{0.294}\\
\bottomrule[1.2pt]

\multirow{5}{*}{\scalebox{1.35}{\rotatebox{90}{ES-LJU}}}
 & \scalebox{1.35}{30} & \scalebox{1.35}{\textbf{0.199}} & \scalebox{1.35}{0.315} & \scalebox{1.35}{0.214} & \scalebox{1.35}{0.330} & \scalebox{1.35}{0.204} & \scalebox{1.35}{0.330} & \scalebox{1.35}{0.218} & \scalebox{1.35}{0.353} & \scalebox{1.35}{0.299} & \scalebox{1.35}{0.433} & \scalebox{1.35}{0.214} & \scalebox{1.35}{0.345} & \scalebox{1.35}{0.230} & \scalebox{1.35}{0.351}  & \scalebox{1.35}{0.489} & \scalebox{1.35}{0.510}  \\
 & \scalebox{1.35}{60} & \scalebox{1.35}{\textbf{0.206}} & \scalebox{1.35}{0.334} & \scalebox{1.35}{0.268} & \scalebox{1.35}{0.364} & \scalebox{1.35}{0.255} & \scalebox{1.35}{0.380} & \scalebox{1.35}{0.256} & \scalebox{1.35}{0.382} & \scalebox{1.35}{0.325} & \scalebox{1.35}{0.453} & \scalebox{1.35}{0.262} & \scalebox{1.35}{0.377} & \scalebox{1.35}{0.292} & \scalebox{1.35}{0.394} & \scalebox{1.35}{0.308} & \scalebox{1.35}{0.407} \\
 & \scalebox{1.35}{90} & \scalebox{1.35}{\textbf{0.245}} & \scalebox{1.35}{0.361} & \scalebox{1.35}{0.304} & \scalebox{1.35}{0.380} & \scalebox{1.35}{0.286} & \scalebox{1.35}{0.394} & \scalebox{1.35}{0.287} & \scalebox{1.35}{0.391} & \scalebox{1.35}{0.319} & \scalebox{1.35}{0.448} & \scalebox{1.35}{0.286} & \scalebox{1.35}{0.393} & \scalebox{1.35}{0.330} & \scalebox{1.35}{0.414} & \scalebox{1.35}{0.336} & \scalebox{1.35}{0.423} \\
 & \scalebox{1.35}{120} & \scalebox{1.35}{\textbf{0.287}} & \scalebox{1.35}{0.393} & \scalebox{1.35}{0.330} & \scalebox{1.35}{0.393} & \scalebox{1.35}{0.304} & \scalebox{1.35}{0.404} & \scalebox{1.35}{0.300} & \scalebox{1.35}{0.405} & \scalebox{1.35}{0.357} & \scalebox{1.35}{0.470} & \scalebox{1.35}{0.304} & \scalebox{1.35}{0.404} & \scalebox{1.35}{0.358} & \scalebox{1.35}{0.430} & \scalebox{1.35}{0.297} & \scalebox{1.35}{0.394} \\
\cmidrule(lr){2-18}
 & \scalebox{1.35}{AVG} & \scalebox{1.35}{\textbf{0.234}} & \scalebox{1.35}{0.351} & \scalebox{1.35}{0.279} & \scalebox{1.35}{0.367} & \scalebox{1.35}{0.262} & \scalebox{1.35}{0.377} & \scalebox{1.35}{0.265} & \scalebox{1.35}{0.383} & \scalebox{1.35}{0.325} & \scalebox{1.35}{0.451} & \scalebox{1.35}{0.267} & \scalebox{1.35}{0.380} & \scalebox{1.35}{0.303} & \scalebox{1.35}{0.397} & \scalebox{1.35}{0.358} & \scalebox{1.35}{0.434} \\
\bottomrule[1.2pt]

\multirow{5}{*}{\scalebox{1.35}{\rotatebox{90}{IT-NOE}}}
& \scalebox{1.35}{30} & \scalebox{1.35}{\textbf{0.320}} & \scalebox{1.35}{0.450} & \scalebox{1.35}{0.335} & \scalebox{1.35}{0.463} & \scalebox{1.35}{0.357} & \scalebox{1.35}{0.478} & \scalebox{1.35}{0.360} & \scalebox{1.35}{0.481} & \scalebox{1.35}{0.374} & \scalebox{1.35}{0.488} & \scalebox{1.35}{0.376} & \scalebox{1.35}{0.485} & \scalebox{1.35}{0.344} & \scalebox{1.35}{0.465} & \scalebox{1.35}{0.473} & \scalebox{1.35}{0.553}\\
 & \scalebox{1.35}{60} & \scalebox{1.35}{\textbf{0.387}} & \scalebox{1.35}{0.486} & \scalebox{1.35}{0.396} & \scalebox{1.35}{0.502} & \scalebox{1.35}{0.426} & \scalebox{1.35}{0.521} & \scalebox{1.35}{0.443} & \scalebox{1.35}{0.531} & \scalebox{1.35}{0.410} & \scalebox{1.35}{0.515} & \scalebox{1.35}{0.480} & \scalebox{1.35}{0.549} & \scalebox{1.35}{0.442} & \scalebox{1.35}{0.528} & \scalebox{1.35}{0.393} & \scalebox{1.35}{0.502}\\
 & \scalebox{1.35}{90} & \scalebox{1.35}{\textbf{0.401}} & \scalebox{1.35}{0.493} & \scalebox{1.35}{0.409} & \scalebox{1.35}{0.508} & \scalebox{1.35}{0.464} & \scalebox{1.35}{0.540} & \scalebox{1.35}{0.461} & \scalebox{1.35}{0.540} & \scalebox{1.35}{0.434} & \scalebox{1.35}{0.525} & \scalebox{1.35}{0.528} & \scalebox{1.35}{0.578} & \scalebox{1.35}{0.502} & \scalebox{1.35}{0.565} & \scalebox{1.35}{0.434} & \scalebox{1.35}{0.534}\\
 & \scalebox{1.35}{120} & \scalebox{1.35}{\textbf{0.388}} & \scalebox{1.35}{0.488} & \scalebox{1.35}{0.421} & \scalebox{1.35}{0.514} & \scalebox{1.35}{0.474} & \scalebox{1.35}{0.551} & \scalebox{1.35}{0.460} & \scalebox{1.35}{0.537} & \scalebox{1.35}{0.415} & \scalebox{1.35}{0.514} & \scalebox{1.35}{0.546} & \scalebox{1.35}{0.588} & \scalebox{1.35}{0.522} & \scalebox{1.35}{0.574} & \scalebox{1.35}{0.456} & \scalebox{1.35}{0.539}\\
\cmidrule(lr){2-18}
 & \scalebox{1.35}{AVG} & \scalebox{1.35}{\textbf{0.374}} & \scalebox{1.35}{0.479} & \scalebox{1.35}{0.390} & \scalebox{1.35}{0.497} & \scalebox{1.35}{0.430} & \scalebox{1.35}{0.523} & \scalebox{1.35}{0.431} & \scalebox{1.35}{0.522} & \scalebox{1.35}{0.408} & \scalebox{1.35}{0.510} & \scalebox{1.35}{0.482} & \scalebox{1.35}{0.550} & \scalebox{1.35}{0.453} & \scalebox{1.35}{0.533} & \scalebox{1.35}{0.439} & \scalebox{1.35}{0.532}\\
\bottomrule[1.2pt]

\multirow{5}{*}{\scalebox{1.35}{\rotatebox{90}{AT-NEU}}}
 & \scalebox{1.35}{30} & \scalebox{1.35}{\textbf{0.290}} & \scalebox{1.35}{0.375} & \scalebox{1.35}{0.316} & \scalebox{1.35}{0.392} & \scalebox{1.35}{0.326} & \scalebox{1.35}{0.415} & \scalebox{1.35}{0.321} & \scalebox{1.35}{0.410} & \scalebox{1.35}{0.326} & \scalebox{1.35}{0.441} & \scalebox{1.35}{0.356} & \scalebox{1.35}{0.448} & \scalebox{1.35}{0.339} & \scalebox{1.35}{0.431} & \scalebox{1.35}{0.555} & \scalebox{1.35}{0.586}\\
 & \scalebox{1.35}{60} & \scalebox{1.35}{\textbf{0.317}} & \scalebox{1.35}{0.407} & \scalebox{1.35}{0.342} & \scalebox{1.35}{0.420} & \scalebox{1.35}{0.354} & \scalebox{1.35}{0.437} & \scalebox{1.35}{0.350} & \scalebox{1.35}{0.430} & \scalebox{1.35}{0.342} & \scalebox{1.35}{0.455} & \scalebox{1.35}{0.391} & \scalebox{1.35}{0.472} & \scalebox{1.35}{0.360} & \scalebox{1.35}{0.446} & \scalebox{1.35}{0.381} & \scalebox{1.35}{0.452}\\
 & \scalebox{1.35}{90} & \scalebox{1.35}{\textbf{0.332}} & \scalebox{1.35}{0.422} & \scalebox{1.35}{0.376} & \scalebox{1.35}{0.454} & \scalebox{1.35}{0.367} & \scalebox{1.35}{0.445} & \scalebox{1.35}{0.369} & \scalebox{1.35}{0.446} & \scalebox{1.35}{0.352} & \scalebox{1.35}{0.466} & \scalebox{1.35}{0.419} & \scalebox{1.35}{0.491} & \scalebox{1.35}{0.380} & \scalebox{1.35}{0.461} & \scalebox{1.35}{0.374} & \scalebox{1.35}{0.440}\\
 & \scalebox{1.35}{120} & \scalebox{1.35}{0.368} & \scalebox{1.35}{0.450} & \scalebox{1.35}{0.422} & \scalebox{1.35}{0.494} & \scalebox{1.35}{0.428} & \scalebox{1.35}{0.493} & \scalebox{1.35}{0.429} & \scalebox{1.35}{0.490} & \scalebox{1.35}{\textbf{0.365}} & \scalebox{1.35}{0.475} & \scalebox{1.35}{0.464} & \scalebox{1.35}{0.520} & \scalebox{1.35}{0.396} & \scalebox{1.35}{0.472} & \scalebox{1.35}{0.424} & \scalebox{1.35}{0.491}\\
\cmidrule(lr){2-18}
 & \scalebox{1.35}{AVG} & \scalebox{1.35}{\textbf{0.327}} & \scalebox{1.35}{0.413} & \scalebox{1.35}{0.364} & \scalebox{1.35}{0.440} & \scalebox{1.35}{0.369} & \scalebox{1.35}{0.448} & \scalebox{1.35}{0.367} & \scalebox{1.35}{0.444} & \scalebox{1.35}{0.346} & \scalebox{1.35}{0.459} & \scalebox{1.35}{0.407} & \scalebox{1.35}{0.483} & \scalebox{1.35}{0.369} & \scalebox{1.35}{0.453} & \scalebox{1.35}{0.434} & \scalebox{1.35}{0.492}\\
\bottomrule[1.2pt]

\multirow{5}{*}{\scalebox{1.35}{\rotatebox{90}{US-LOS}}}
 & \scalebox{1.35}{30} & \scalebox{1.35}{0.204} & \scalebox{1.35}{0.190} & \scalebox{1.35}{0.281} & \scalebox{1.35}{0.237} & \scalebox{1.35}{0.248} & \scalebox{1.35}{0.199} & \scalebox{1.35}{0.250} & \scalebox{1.35}{0.199} & \scalebox{1.35}{0.720} & \scalebox{1.35}{0.578} & \scalebox{1.35}{\textbf{0.177}} & \scalebox{1.35}{0.333} & \scalebox{1.35}{0.210} & \scalebox{1.35}{0.185} & \scalebox{1.35}{0.405} & \scalebox{1.35}{0.278}\\
 & \scalebox{1.35}{60} & \scalebox{1.35}{\textbf{0.305}} & \scalebox{1.35}{0.231} & \scalebox{1.35}{0.383} & \scalebox{1.35}{0.262} & \scalebox{1.35}{0.377} & \scalebox{1.35}{0.246} & \scalebox{1.35}{0.365} & \scalebox{1.35}{0.246} & \scalebox{1.35}{0.770} & \scalebox{1.35}{0.624} & \scalebox{1.35}{0.397} & \scalebox{1.35}{0.508} & \scalebox{1.35}{0.345} & \scalebox{1.35}{0.238} & \scalebox{1.35}{0.381} & \scalebox{1.35}{0.277}\\
 & \scalebox{1.35}{90} & \scalebox{1.35}{\textbf{0.421}} & \scalebox{1.35}{0.268} & \scalebox{1.35}{0.465} & \scalebox{1.35}{0.280} & \scalebox{1.35}{0.478} & \scalebox{1.35}{0.290} & \scalebox{1.35}{0.507} & \scalebox{1.35}{0.309} & \scalebox{1.35}{0.765} & \scalebox{1.35}{0.621} & \scalebox{1.35}{0.619} & \scalebox{1.35}{0.668} & \scalebox{1.35}{0.449} & \scalebox{1.35}{0.276} & \scalebox{1.35}{0.520} & \scalebox{1.35}{0.297}\\
 & \scalebox{1.35}{120} & \scalebox{1.35}{\textbf{0.509}} & \scalebox{1.35}{0.293} & \scalebox{1.35}{0.547} & \scalebox{1.35}{0.306} & \scalebox{1.35}{0.571} & \scalebox{1.35}{0.314} & \scalebox{1.35}{0.589} & \scalebox{1.35}{0.332} & \scalebox{1.35}{0.782} & \scalebox{1.35}{0.624} & \scalebox{1.35}{0.851} & \scalebox{1.35}{0.810} & \scalebox{1.35}{0.531} & \scalebox{1.35}{0.305} & \scalebox{1.35}{0.558} & \scalebox{1.35}{0.330}\\
\cmidrule(lr){2-18}
 & \scalebox{1.35}{AVG} & \scalebox{1.35}{\textbf{0.360}} & \scalebox{1.35}{0.245} & \scalebox{1.35}{0.419} & \scalebox{1.35}{0.271} & \scalebox{1.35}{0.418} & \scalebox{1.35}{0.262} & \scalebox{1.35}{0.428} & \scalebox{1.35}{0.272} & \scalebox{1.35}{0.759} & \scalebox{1.35}{0.612} & \scalebox{1.35}{0.511} & \scalebox{1.35}{0.580} & \scalebox{1.35}{0.384} & \scalebox{1.35}{0.251} & \scalebox{1.35}{0.466} & \scalebox{1.35}{0.296}\\
\bottomrule[1.2pt]

\end{tabular}}
\label{tab:flux_tower_results}
\end{sc}
\end{table}

\begin{table}[h]
\caption{Full results of the long-term forecasting with exogenous variables task. STREAMFLOW}
\vspace{2pt}
\setlength{\tabcolsep}{2.5pt}

\begin{sc}
\resizebox{\linewidth}{!}{
\begin{tabular}{c|c|cc|cc|cc|cc|cc|cc}
\toprule[1.2pt]  
\multicolumn{2}{c}{\multirow{2}{*}{\scalebox{1.35}{Models}}}   & \multicolumn{2}{c}{\scalebox{1.35}{FutureTST}} & \multicolumn{2}{c}{\scalebox{1.35}{iTrans.}} & \multicolumn{2}{c}{\scalebox{1.35}{(U)PatchTST}} & \multicolumn{2}{c}{\scalebox{1.35}{(M)PatchTST}} & \multicolumn{2}{c}{\scalebox{1.35}{LSTM}} & \multicolumn{2}{c}{\scalebox{1.35}{DLinear}} \\ 
\multicolumn{2}{c}{} & \multicolumn{2}{c}{\scalebox{1.35}{(Ours)}} & \multicolumn{2}{c}{\scalebox{1.35}{\citeyearpar{liu2023itransformer}}} & \multicolumn{2}{c}{\scalebox{1.35}{\citeyearpar{li2023revisiting}}} & \multicolumn{2}{c}{\scalebox{1.35}{\citeyearpar{nie2022time}}} & \multicolumn{2}{c}{\scalebox{1.35}{\citeyearpar{zhang2022crossformer}}} & \multicolumn{2}{c}{\scalebox{1.35}{\citeyearpar{das2023long}}}  \\ 
\cmidrule(lr){3-4}\cmidrule(lr){5-6}\cmidrule(lr){7-8}\cmidrule(lr){9-10}\cmidrule(lr){11-12}\cmidrule(lr){13-14}
\multicolumn{2}{c}{\scalebox{1.35}{Metric}}   & \scalebox{1.35}{MSE} & \scalebox{1.35}{MAE} & \scalebox{1.35}{MSE}    & \scalebox{1.35}{MAE}   & \scalebox{1.35}{MSE}    & \scalebox{1.35}{MAE}    & \scalebox{1.35}{MSE}    & \scalebox{1.35}{MAE} & \scalebox{1.35}{MSE}    & \scalebox{1.35}{MAE} & \scalebox{1.35}{MSE}    & \scalebox{1.35}{MAE}         \\ 
\toprule[1.2pt] 
\multirow{5}{*}{\scalebox{1.35}{\rotatebox{90}{ECL}}}
 & \scalebox{1.35}{30} & \scalebox{1.35}{0.693} & \scalebox{1.35}{0.306} & \scalebox{1.35}{1.087} & \scalebox{1.35}{0.288} & \scalebox{1.35}{1.123} & \scalebox{1.35}{0.377} & \scalebox{1.35}{1.121} & \scalebox{1.35}{0.386} & \scalebox{1.35}{0.452} & \scalebox{1.35}{0.244} & \scalebox{1.35}{1.111} & \scalebox{1.35}{0.373} \\
 & \scalebox{1.35}{60} & \scalebox{1.35}{0.788} & \scalebox{1.35}{0.311} & \scalebox{1.35}{1.096} & \scalebox{1.35}{0.290} & \scalebox{1.35}{1.156} & \scalebox{1.35}{0.411} & \scalebox{1.35}{1.152} & \scalebox{1.35}{0.390} & \scalebox{1.35}{0.474} & \scalebox{1.35}{0.251} & \scalebox{1.35}{1.133} & \scalebox{1.35}{0.381} \\
 & \scalebox{1.35}{90} & \scalebox{1.35}{0.855} & \scalebox{1.35}{0.320} & \scalebox{1.35}{1.091} & \scalebox{1.35}{0.281} & \scalebox{1.35}{1.164} & \scalebox{1.35}{0.404} & \scalebox{1.35}{1.168} & \scalebox{1.35}{0.406} & \scalebox{1.35}{0.481} & \scalebox{1.35}{0.255} & \scalebox{1.35}{1.156} & \scalebox{1.35}{0.393} \\
 & \scalebox{1.35}{120} & \scalebox{1.35}{0.882} & \scalebox{1.35}{0.326} & \scalebox{1.35}{1.095} & \scalebox{1.35}{0.290} & \scalebox{1.35}{1.186} & \scalebox{1.35}{0.407} & \scalebox{1.35}{1.180} & \scalebox{1.35}{0.405} & \scalebox{1.35}{0.477} & \scalebox{1.35}{0.255} & \scalebox{1.35}{1.169} & \scalebox{1.35}{0.398} \\
\cmidrule(lr){2-14}
 & \scalebox{1.35}{AVG} & \scalebox{1.35}{0.804} & \scalebox{1.35}{0.316} & \scalebox{1.35}{1.092} & \scalebox{1.35}{0.287} & \scalebox{1.35}{1.157} & \scalebox{1.35}{0.400} & \scalebox{1.35}{1.155} & \scalebox{1.35}{0.397} & \scalebox{1.35}{0.471} & \scalebox{1.35}{0.251} & \scalebox{1.35}{1.142} & \scalebox{1.35}{0.386} \\
\bottomrule[1.2pt]

\multirow{5}{*}{\scalebox{1.35}{\rotatebox{90}{ECL}}}
 & \scalebox{1.35}{30} & \scalebox{1.35}{0.475} & \scalebox{1.35}{0.375} & \scalebox{1.35}{0.914} & \scalebox{1.35}{0.499} & \scalebox{1.35}{0.875} & \scalebox{1.35}{0.516} & \scalebox{1.35}{0.883} & \scalebox{1.35}{0.521} & \scalebox{1.35}{0.303} & \scalebox{1.35}{0.256} & \scalebox{1.35}{0.871} & \scalebox{1.35}{0.496} \\
 & \scalebox{1.35}{60} & \scalebox{1.35}{0.530} & \scalebox{1.35}{0.402} & \scalebox{1.35}{0.892} & \scalebox{1.35}{0.493} & \scalebox{1.35}{0.941} & \scalebox{1.35}{0.526} & \scalebox{1.35}{0.906} & \scalebox{1.35}{0.519} & \scalebox{1.35}{0.286} & \scalebox{1.35}{0.252} & \scalebox{1.35}{0.893} & \scalebox{1.35}{0.507} \\
 & \scalebox{1.35}{90} & \scalebox{1.35}{0.536} & \scalebox{1.35}{0.401} & \scalebox{1.35}{0.879} & \scalebox{1.35}{0.497} & \scalebox{1.35}{0.914} & \scalebox{1.35}{0.538} & \scalebox{1.35}{0.919} & \scalebox{1.35}{0.530} & \scalebox{1.35}{0.290} & \scalebox{1.35}{0.250} & \scalebox{1.35}{0.902} & \scalebox{1.35}{0.513} \\
 & \scalebox{1.35}{120} & \scalebox{1.35}{0.566} & \scalebox{1.35}{0.420} & \scalebox{1.35}{0.877} & \scalebox{1.35}{0.497} & \scalebox{1.35}{0.930} & \scalebox{1.35}{0.534} & \scalebox{1.35}{0.920} & \scalebox{1.35}{0.526} & \scalebox{1.35}{0.306} & \scalebox{1.35}{0.256} & \scalebox{1.35}{0.908} & \scalebox{1.35}{0.513} \\
\cmidrule(lr){2-14}
 & \scalebox{1.35}{AVG} & \scalebox{1.35}{0.527} & \scalebox{1.35}{0.399} & \scalebox{1.35}{0.891} & \scalebox{1.35}{0.496} & \scalebox{1.35}{0.915} & \scalebox{1.35}{0.528} & \scalebox{1.35}{0.907} & \scalebox{1.35}{0.524} & \scalebox{1.35}{0.296} & \scalebox{1.35}{0.254} & \scalebox{1.35}{0.893} & \scalebox{1.35}{0.507} \\
\bottomrule[1.2pt]

\multirow{5}{*}{\scalebox{1.35}{\rotatebox{90}{ECL}}}
 & \scalebox{1.35}{30} & \scalebox{1.35}{0.380} & \scalebox{1.35}{0.159} & \scalebox{1.35}{0.387} & \scalebox{1.35}{0.158} & \scalebox{1.35}{0.413} & \scalebox{1.35}{0.187} & \scalebox{1.35}{0.420} & \scalebox{1.35}{0.190} & \scalebox{1.35}{0.274} & \scalebox{1.35}{0.148} & \scalebox{1.35}{0.408} & \scalebox{1.35}{0.197} \\
 & \scalebox{1.35}{60} & \scalebox{1.35}{0.390} & \scalebox{1.35}{0.160} & \scalebox{1.35}{0.385} & \scalebox{1.35}{0.155} & \scalebox{1.35}{0.451} & \scalebox{1.35}{0.221} & \scalebox{1.35}{0.441} & \scalebox{1.35}{0.210} & \scalebox{1.35}{0.264} & \scalebox{1.35}{0.145} & \scalebox{1.35}{0.412} & \scalebox{1.35}{0.204} \\
 & \scalebox{1.35}{90} & \scalebox{1.35}{0.406} & \scalebox{1.35}{0.177} & \scalebox{1.35}{0.391} & \scalebox{1.35}{0.158} & \scalebox{1.35}{0.428} & \scalebox{1.35}{0.194} & \scalebox{1.35}{0.429} & \scalebox{1.35}{0.197} & \scalebox{1.35}{0.282} & \scalebox{1.35}{0.153} & \scalebox{1.35}{0.416} & \scalebox{1.35}{0.213} \\
 & \scalebox{1.35}{120} & \scalebox{1.35}{0.410} & \scalebox{1.35}{0.173} & \scalebox{1.35}{0.386} & \scalebox{1.35}{0.150} & \scalebox{1.35}{0.468} & \scalebox{1.35}{0.235} & \scalebox{1.35}{0.445} & \scalebox{1.35}{0.212} & \scalebox{1.35}{0.289} & \scalebox{1.35}{0.164} & \scalebox{1.35}{0.420} & \scalebox{1.35}{0.220} \\
\cmidrule(lr){2-14}
 & \scalebox{1.35}{AVG} & \scalebox{1.35}{0.397} & \scalebox{1.35}{0.167} & \scalebox{1.35}{0.387} & \scalebox{1.35}{0.155} & \scalebox{1.35}{0.440} & \scalebox{1.35}{0.209} & \scalebox{1.35}{0.434} & \scalebox{1.35}{0.202} & \scalebox{1.35}{0.277} & \scalebox{1.35}{0.152} & \scalebox{1.35}{0.414} & \scalebox{1.35}{0.208} \\
\bottomrule[1.2pt]

\multirow{5}{*}{\scalebox{1.35}{\rotatebox{90}{ECL}}}
 & \scalebox{1.35}{30} & \scalebox{1.35}{0.298} & \scalebox{1.35}{0.190} & \scalebox{1.35}{0.363} & \scalebox{1.35}{0.215} & \scalebox{1.35}{0.435} & \scalebox{1.35}{0.335} & \scalebox{1.35}{0.416} & \scalebox{1.35}{0.310} & \scalebox{1.35}{0.183} & \scalebox{1.35}{0.196} & \scalebox{1.35}{0.381} & \scalebox{1.35}{0.263} \\
 & \scalebox{1.35}{60} & \scalebox{1.35}{0.330} & \scalebox{1.35}{0.202} & \scalebox{1.35}{0.367} & \scalebox{1.35}{0.219} & \scalebox{1.35}{0.467} & \scalebox{1.35}{0.360} & \scalebox{1.35}{0.463} & \scalebox{1.35}{0.350} & \scalebox{1.35}{0.180} & \scalebox{1.35}{0.188} & \scalebox{1.35}{0.389} & \scalebox{1.35}{0.273} \\
 & \scalebox{1.35}{90} & \scalebox{1.35}{0.338} & \scalebox{1.35}{0.210} & \scalebox{1.35}{0.375} & \scalebox{1.35}{0.228} & \scalebox{1.35}{0.474} & \scalebox{1.35}{0.355} & \scalebox{1.35}{0.494} & \scalebox{1.35}{0.379} & \scalebox{1.35}{0.178} & \scalebox{1.35}{0.185} & \scalebox{1.35}{0.395} & \scalebox{1.35}{0.278} \\
 & \scalebox{1.35}{120} & \scalebox{1.35}{0.344} & \scalebox{1.35}{0.205} & \scalebox{1.35}{0.381} & \scalebox{1.35}{0.223} & \scalebox{1.35}{0.463} & \scalebox{1.35}{0.346} & \scalebox{1.35}{0.479} & \scalebox{1.35}{0.362} & \scalebox{1.35}{0.184} & \scalebox{1.35}{0.189} & \scalebox{1.35}{0.400} & \scalebox{1.35}{0.288} \\
\cmidrule(lr){2-14}
 & \scalebox{1.35}{AVG} & \scalebox{1.35}{0.328} & \scalebox{1.35}{0.202} & \scalebox{1.35}{0.371} & \scalebox{1.35}{0.221} & \scalebox{1.35}{0.460} & \scalebox{1.35}{0.349} & \scalebox{1.35}{0.463} & \scalebox{1.35}{0.350} & \scalebox{1.35}{0.181} & \scalebox{1.35}{0.190} & \scalebox{1.35}{0.391} & \scalebox{1.35}{0.276} \\
\bottomrule[1.2pt]
\multirow{5}{*}{\scalebox{1.35}{\rotatebox{90}{ECL}}}
 & \scalebox{1.35}{30} & \scalebox{1.35}{0.613} & \scalebox{1.35}{0.357} & \scalebox{1.35}{0.969} & \scalebox{1.35}{0.380} & \scalebox{1.35}{1.023} & \scalebox{1.35}{0.451} & \scalebox{1.35}{1.019} & \scalebox{1.35}{0.454} & \scalebox{1.35}{0.394} & \scalebox{1.35}{0.287} & \scalebox{1.35}{1.013} & \scalebox{1.35}{0.437} \\
 & \scalebox{1.35}{60} & \scalebox{1.35}{0.680} & \scalebox{1.35}{0.384} & \scalebox{1.35}{0.972} & \scalebox{1.35}{0.361} & \scalebox{1.35}{1.032} & \scalebox{1.35}{0.443} & \scalebox{1.35}{1.032} & \scalebox{1.35}{0.451} & \scalebox{1.35}{0.404} & \scalebox{1.35}{0.295} & \scalebox{1.35}{1.026} & \scalebox{1.35}{0.440} \\
 & \scalebox{1.35}{90} & \scalebox{1.35}{0.703} & \scalebox{1.35}{0.386} & \scalebox{1.35}{0.949} & \scalebox{1.35}{0.368} & \scalebox{1.35}{1.018} & \scalebox{1.35}{0.451} & \scalebox{1.35}{1.014} & \scalebox{1.35}{0.443} & \scalebox{1.35}{0.382} & \scalebox{1.35}{0.294} & \scalebox{1.35}{1.008} & \scalebox{1.35}{0.441} \\
 & \scalebox{1.35}{120} & \scalebox{1.35}{0.707} & \scalebox{1.35}{0.383} & \scalebox{1.35}{0.916} & \scalebox{1.35}{0.362} & \scalebox{1.35}{0.990} & \scalebox{1.35}{0.458} & \scalebox{1.35}{0.982} & \scalebox{1.35}{0.439} & \scalebox{1.35}{0.388} & \scalebox{1.35}{0.293} & \scalebox{1.35}{0.977} & \scalebox{1.35}{0.443} \\
\cmidrule(lr){2-14}
 & \scalebox{1.35}{AVG} & \scalebox{1.35}{0.676} & \scalebox{1.35}{0.378} & \scalebox{1.35}{0.951} & \scalebox{1.35}{0.368} & \scalebox{1.35}{1.016} & \scalebox{1.35}{0.451} & \scalebox{1.35}{1.012} & \scalebox{1.35}{0.447} & \scalebox{1.35}{0.392} & \scalebox{1.35}{0.292} & \scalebox{1.35}{1.006} & \scalebox{1.35}{0.440} \\
\bottomrule[1.2pt]

\end{tabular}}
\label{tab:full-log}
\end{sc}
\end{table}

\subsection{Implementation details} \label{appendix:implementation_details}

We divided the dataset into three consecutive time windows for training (70\%), validation (10\%), and testing (20\%). Training utilized earlier timesteps, while later timesteps were reserved for testing. All models were trained using mean square error loss, capped at a maximum of 20 epochs, employing Adam optimizers with early stopping triggered by validation performance. To ensure fairness, the training, validation, and testing datasets were standardized across all models to eliminate biases in model comparisons. Every model, including ours, had a consistent lookback period of 512 days, with forecasting periods set at 30, 60, 90, and 120 days. For our model, we configured a patch length of 16 and a stride of 8.

\subsection{Baseline Models}\label{appendix:baseline_models}
To robustly assess the efficacy of our proposed methodology for long-term temporal modeling, we compare it against a  six state-of-the-art time series forecasting models prevalent in recent literature:

\begin{itemize}
    \item \textbf{Transformer-based Models:} 
    \begin{itemize}
        \item \textbf{iTransformer} \cite{liu2023itransformer}: This approach applies the attention and feed-forward network mechanisms across inverted dimensions. Specifically, the time points in each individual series are transformed into variate tokens. These tokens are then processed by the attention mechanism, enabling the capture of multivariate correlations. Concurrently, the feed-forward network is employed on each variate token individually to derive nonlinear representations.

        \item \textbf{(U)PatchTST} \cite{nie2022time}: This model segments time series data into patches processed by a Transformer. The "(U)" indicates a univariate approach, focusing solely on past endogenous series for future predictions, without incorporating exogenous variables.

        \item \textbf{(M)PatchTST} \cite{nie2022time}: Operating under the same patching principles as PatchTST, the "(M)" denotes a multivariate method. This variant utilizes both past exogenous and endogenous series to forecast both future endogenous and exogenous series.
        
    \end{itemize}
    \item \textbf{Linear Models:}
    \begin{itemize}
        \item \textbf{DLinear} \cite{zeng2023transformers}:  is a simple one-layer linear model designed for long-term time series forecasting.
    \end{itemize}
    \item \textbf{State Space Model:}
    \begin{itemize}
        \item \textbf{S-MAMBA} \cite{wang2024mamba}: Mamba, a selective state space model, has gained traction due to its ability to process dependencies in sequences while maintaining near-linear complexity. Its derivative, Simple-Mamba (S-Mamba), tokenizes each variate's time points independently using a linear layer for time series forecasting and uses a bidirectional Mamba layer to capture inter-variate correlations. 
    \end{itemize}
    \item \textbf{Multilayer Perceptron-based Model:}
    \begin{itemize}
        \item \textbf{TiDE} \cite{das2023long}: Time-series Dense Encoder (TiDE) model offers a  MLP-based encoder-decoder architecture that can efficiently  handles past, future exogenous driver using dense MLP. 
    \end{itemize}
    \item \textbf{Long Short-Term Memory (LSTM) Model} : 
    \begin{itemize}
    \item  \textbf{Encoder-decoder LSTM} \cite{hochreiter1997long,yin2022rr} model involves two main components. The encoder processes past exogenous and endogenous variables, capturing the data's temporal dynamics. This encoder generates a hidden state and a cell state, which are then passed to the LSTM decoder. The decoder uses these states, along with future exogenous inputs, to predict future values of the endogenous variables.
    \end{itemize}

\end{itemize}
 For all baselines, we used default parameters for all baselines as described in their original paper. \textbf{TiDE and LSTM are the sole baselines that are able to utilize future exogenous inputs.}

\subsection{Flux Tower TimeSeries}\label{appendix:flux_dataset}
Here we present the time series for Gross Primary Production (GPP) across five distinct ecological regions used in our study. The original dataset from US-LOS contained missing values that were filled using linear interpolation, leading to irregularities observed in its time series graph.

\begin{figure*}[t]
    \centering
    \includegraphics[width=0.5\linewidth]{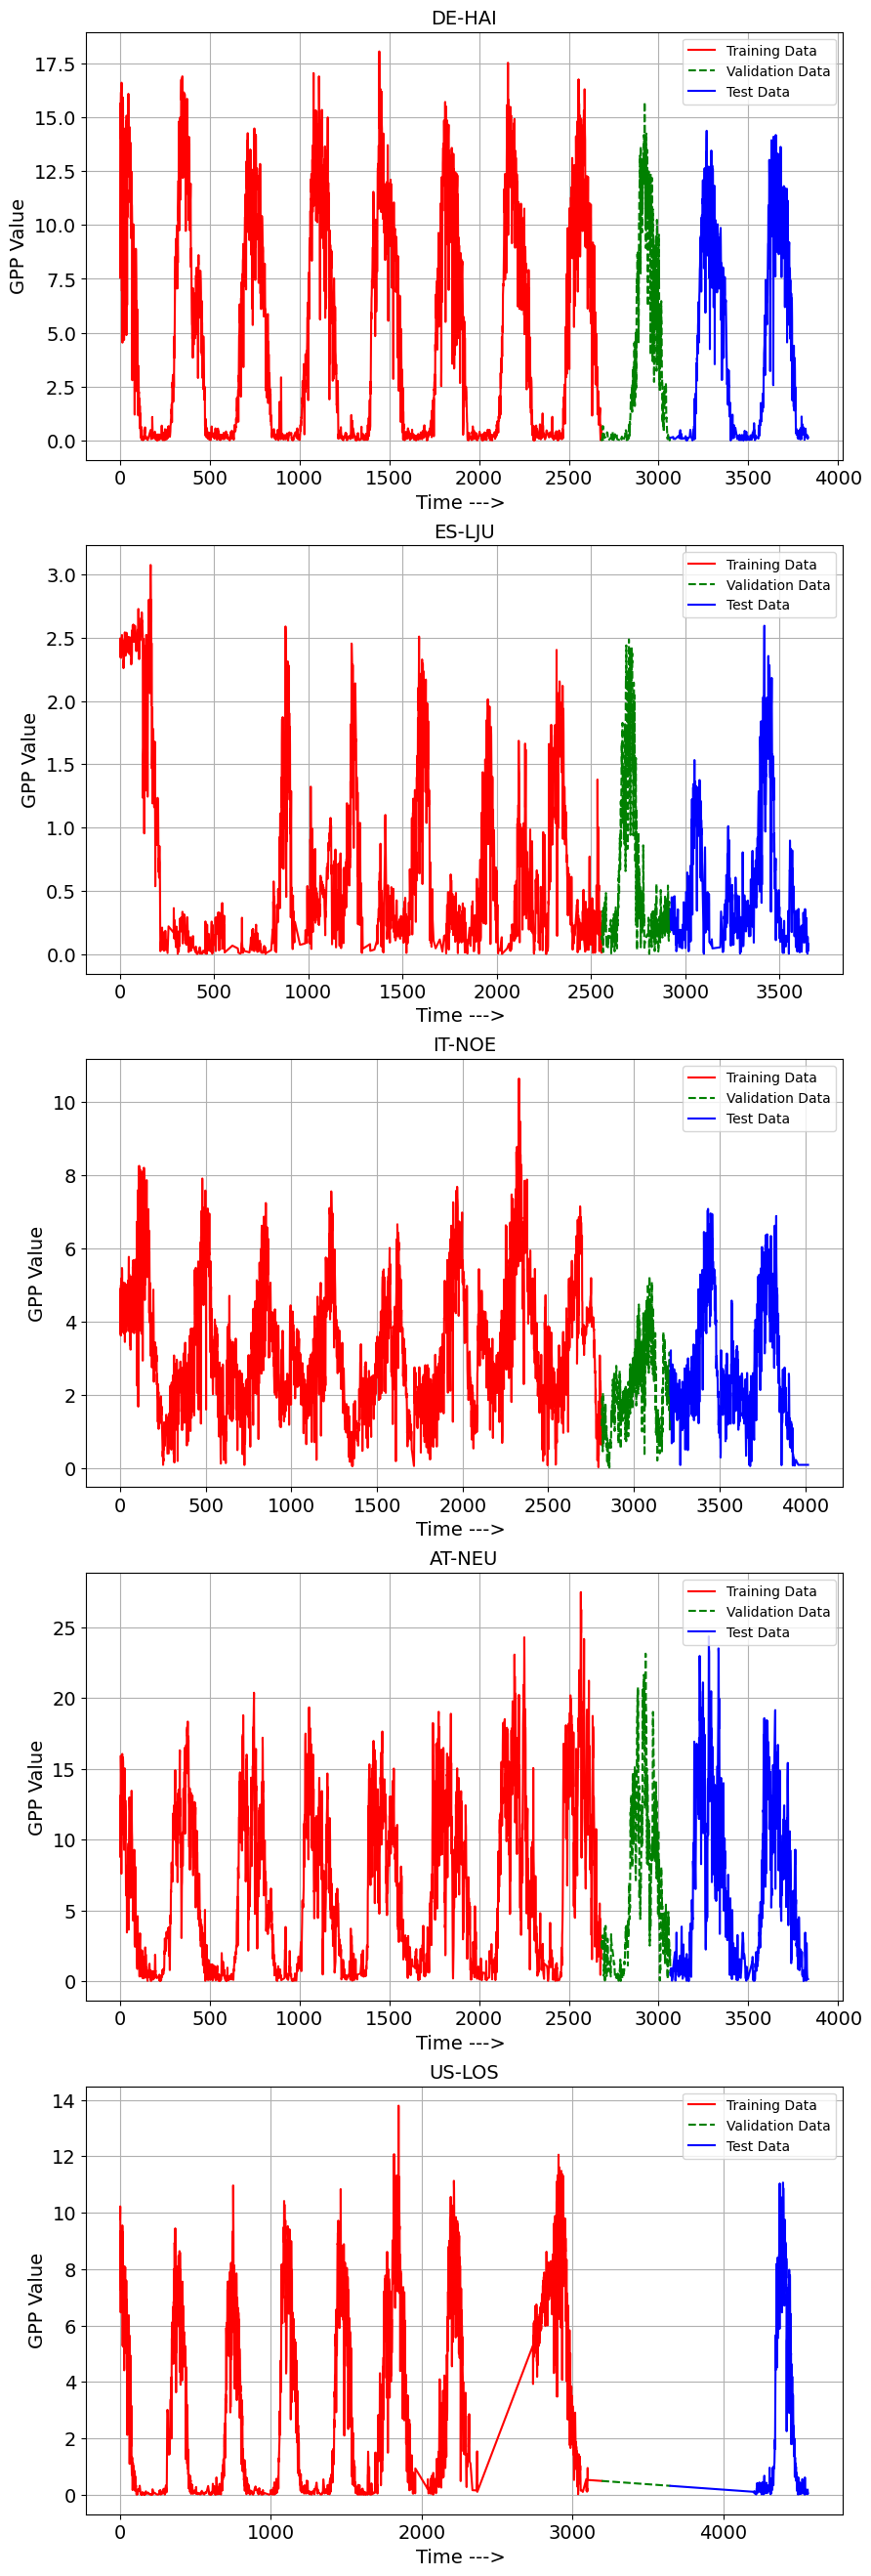} % Adjust width as needed
    \caption{\footnotesize} % Adjust font size as needed
    \label{fig:flux_dataset}
    \vspace{-0.2cm} % Adjust vertical space as needed
\end{figure*}
